# Supplementary material for: Nested replicator dynamics, nested logit choice, and similarity-based learning
Source: arXiv:2407.17815 source file (2024-07-25)
Supplement: Supplementary file 1 [file App-Defs.tex]

%----------------------------------------------------------------------
%%% APP: DEFINITIONS
%----------------------------------------------------------------------
% !TEX root = ../Main.tex


In this appendix, we provide some definitions from dynamical systems that were omitted from the main text.
To state them, consider a dynamical system of the form
\begin{equation}
\label{eq:dyn}
\tag{D}
\dot\strat
	= \dynfield(\strat),
\end{equation}
where the \emph{motion field} $\dynfield\from\strats\to\R^{\nElems}$ is assumed to satisfy the feasibility condition $\dynfield(\strat) \in \tcone_{\strat}\strats$, where $\tcone_{\strat}\strats$ denotes the \emph{tangent cone} to $\strats$ at $\strat$, \viz
\begin{equation}
\label{eq:cone}
\tcone_{\strat}\strats
	= \setdef*
	{\pvec\in\R^{\elems}}
	{\text{$\insum_{\elem\in\elems} \pvec_{\elem} = 0$ and $\pvec_{\elem}\geq0$ whenever $\strat_{\elem}=0$}}.
\end{equation}
Under this condition, Lipschitz continuity of $\dynfield(\strat)$ ensures that the system \eqref{eq:dyn} is \emph{well-posed}, i.e. it admits unique solutions that exist for all time from any initial condition $\orbit{\tstart}\in\strats$.
If, in addition, $\dynfield$ satisfies the more restrictive tangency condition $\dynfield(\strat) \in \tspace_{\strat}\strats$ where
\begin{equation}
\label{eq:tangent}
\tspace_{\strat}\strats
	= \setdef*
	{\pvec\in\R^{\elems}}
	{\text{$\insum_{\elem\in\elems} \pvec_{\elem} = 0$ and $\pvec_{\elem}=$ whenever $\strat_{\elem}=0$}}
\end{equation}
denotes the \emph{tangent space} to $\strats$ at $\strat$, it is straighforward to verify that the faces of $\strats$ remain invariant under \eqref{eq:dyn},
%support of any solution orbit $\orbit{\time}$ of \eqref{eq:dyn} remains invariant under \eqref{eq:dyn},
\ie $\supp(\orbit{\time}) = \supp(\orbit{\tstart})$ for all $\time\geq0$.

When \eqref{eq:dyn} is well-posed, we have the following series of definitions regarding notions of stationarity, stability, and convergence:

\begin{definition}
\label{def:dynamics}
Let \eqref{eq:dyn} be a well-posed dynamical system on $\strats$.
%and let $(\orbit{\time})_{t\geq0}$ be a \textpar{global} solution thereof.
Then:
\begin{enumerate}

\item
$\olim\in\strats$ is said to be an \emph{$\omega$-limit} of a solution $\orbit{\time}$ of \eqref{eq:dyn} if there exists an increasing sequence of times $\time_{\run}\uparrow\infty$ such that $\lim_{\run\to\infty} \orbit{\time_{\run}} = \olim$.

\item
$\eq\in\strats$ is \emph{\textpar{Lyapunov} stable} if, for every neighborhood $\nhd$ of $\eq$ in $\strats$, there exists a neighborhood $\alt\nhd$ of $\eq$ such that every solution $\orbit{\time}$ of \eqref{eq:dyn} that starts in $\alt\nhd$ remains in $\nhd$ for all $t\geq0$.

\item
$\eq\in\strats$ is \emph{attracting} if there exists a neighborhood $\nhd$ of $\eq$ in $\strats$ such that every solution $\orbit{\time}$ of \eqref{eq:dyn} that starts in $\nhd$ converges to $\eq$ as $t\to\infty$.

\item
$\eq\in\strats$ is \emph{asymptotically stable} if it is both stable and attracting.
\end{enumerate}
\end{definition}

The Lipschitz and tangency requirements above are both easy to check for \eqref{eq:NRD}, so the well-posedness and face invariance properties of \eqref{eq:NRD} follow directly.
In view of this, we will apply the above definitions to \eqref{eq:NRD} without further qualifications.

%\PM{Discuss here well-posedness of \eqref{eq:NRD}.}
%\WHS{Also invariance of support of $\orbit{\time}$.}
%\PM{Duly noted.}
